# Supplementary material for: Fundamental Limits of Online Network-Caching
Source: arXiv:2003.14085 source file (2020-03-31)
Supplement: Supplementary file 1 [file appendix.tex]

\section{Appendix}

\subsection{Proof of Theorem \ref{reg_lb_gnl}}
\begin{proof}
%Next, we return to the proof of the regret lower bounds for the library size $N$ and cache capacity $C$, where a user may request upto $r \leq C$ files at a time. 
As in the proof of Theorem \ref{reg_lb_spl}, let the caching decisions made by any admissible single-server caching policy at time $t$ be given by the vector $\bm{y}_t \in [0,1]^N$. The interpretation of $\bm{y}_t$ is that $y_{ti}$ denotes the fraction of the $i$\textsuperscript{th} file decided to be cached by the policy. Any admissible caching policy must respect the following cache-capacity constraint: 
\begin{eqnarray} \label{cache-capacity}
0 \leq \sum_i y_{ti} \leq C, ~~\forall t.
\end{eqnarray}
Let $\bm{x}_t$ be the incoming file request vector at time $t$ such that $x_{ti}$ denotes the number of requests for the file $i$ at time $t$. 
%Note that there could be multiple requests for a single file, presumably coming from two different users. \\
%\footnote{Our proof goes through even when the variables $x_{ti}$ and $y_{ti}$ are fractional. This is relevant to the situation when the users are interested in parts of a file (say the trailer of a new movie).}. 
Clearly,

\[0 \leq \sum_i x_{ti} \leq r,~~ \forall~ t. \]
% We need to lower bound the regret as defined below:  
%\begin{eqnarray} \label{regret_def}
%R_T=\sup_{\{\bm{x}_t\}_{t=1}^{T}} \sup_{\bm{y^*}}\bigg({\bm{y^*}}'\sum_{t=1}^{T} \bm{x}_t - \sum_{t=1}^{T} \bm{y}_t' \bm{x}_t\bigg). 
%\end{eqnarray}
For a given file request sequence $\{\bm{x}_t\}_{t=1}^{T}$, an optimal \emph{offline} static cache configuration vector $\bm{y}^* \in [0,1]^N,$ yielding the highest reward \eqref{reward_def}, simply sets the coordinates corresponding to the \emph{maximum $C$ coordinates} of the $N$-dimensional vector $\sum_{t=1}^{T} \bm{x}_t$ to unity. \\
To lower bound the regret $R_T^\pi$ in equation \eqref{regret_def}, we consider a random request sequence $\bm{X}_t$, sampled independently (across time) as follows 
\[\bm{X}_t = \sum_{k=1}^{r} \bm{E}_{tk},\] 
where the random variable $\bm{E}_{tk}$ is sampled independently and uniformly at random from the set of first $2C$ unit vectors $\{\bm{e}_i, 1\leq i \leq 2C\}$. Recall that, the unit vector $\bm{e}_i$ has one at its $i$\textsuperscript{th} coordinate and zeros everywhere else. With this, the expected value of the second term in Eqn.\ \eqref{regret_def} is easy to compute: 
\begin{eqnarray} \label{ex2}
\mathbb{E}\bigg(\sum_{t=1}^{T} \bm{Y}_t \cdot \bm{X}_t\bigg) &\stackrel{(a)}{=}& \sum_{t=1}^{T}\bm{Y}_t \cdot \big(\mathbb{E}\bm{X}_t\big) \nonumber \\
&=& \frac{r}{2C}\sum_{t=1}^{T} \sum_{k=1}^{2C}\bm{Y}_{tk}  
 \stackrel{(b)}{\leq} \frac{rT}{2}, 
\end{eqnarray}
where, in (a), we have used the fact that the caching decision $\bm{Y}_t$ made at time $t$ is independent of the request vector $\bm{X}_t$, and in (b) we have used the cache-capacity constraint \eqref{cache-capacity}, as for all $t$:
\[\sum_{k=1}^{2C}\bm{Y}_{tk} \leq \sum_{k=1}^{N} \bm{Y}_{tk} \leq C. \]
Finally, we evaluate the expectation of the first term. As argued before, the random variable ${\bm{Y^*}}\cdot \sum_{t=1}^{T} \bm{X}_t$ is identically distributed as the total number of balls in the highest loaded $C$ bins when $m=rT$ balls are randomly thrown into $2C$ bins. Hence, using Lemma \ref{max_load}, we have 
\begin{eqnarray} \label{ex1}
\mathbb{E}\bigg({\bm{Y^*}} \cdot \sum_{t=1}^{T} \bm{X}_t\bigg) \geq \frac{rT}{2}+ \sqrt{\frac{rCT}{2\pi}} - \Theta(\frac{1}{\sqrt{T}}).
\end{eqnarray}
Combining equations \eqref{ex2} and \eqref{ex1}, we have that 
\begin{eqnarray} \label{reg_bd}
&& \mathbb{E}_{\{\bm{X}_t\}_{t=1}^{T}}\bigg({\bm{Y^*}}\cdot \sum_{t=1}^{T} \bm{X}_t - \sum_{t=1}^{T}\bm{Y}_t \cdot \bm{X}_t \bigg) \nonumber \\
&\geq&  \sqrt{\frac{rCT}{2\pi}}- \Theta(\frac{1}{\sqrt{T}}).
\end{eqnarray}
 Inequality \eqref{reg_bd} concludes the proof of Theorem \ref{reg_lb_gnl}. 

\end{proof}

\subsection{Proof of Theorem \ref{elastic_th}} \label{reg_bd_elastic}
\begin{proof}
Let $\bm{x}_t^{i}$ be the file request vector from the $i$\textsuperscript{th} user, and $\bm{y}_t^{j}$ be the cache configuration vector of the $j$\textsuperscript{th} cache set by policy $\pi$ at time $t$, where $i \in \mathcal{I}, j \in \mathcal{J}$. Hence, due to the elastic nature of the content, the total reward $G^\pi_T$ accrued by the caching policy $\pi$ is given by Eqn.\ \eqref{elastic_content}: 
%\footnote{We consider the case of caching with multiple layers of coding (\emph{e.g.,} HDTV) where the user experience increases with increased amount of cached content. When this assumption does not hold, we need to cap the per-time slot gain of each user by $1$, i.e. the term within the summation would be $\min (1, \bm{x}^i_t \cdot \sum_{j\in \delta^+(i)}\bm{y}_t^j) $.}
\[ G_T^\pi = \sum_{t=1}^{T} \sum_{i \in \mathcal{I}} \bm{x}^i_t \cdot \sum_{j\in \partial^+(i)}\bm{y}_t^j.\]
Recall that, to compute the regret, we compare the reward of the caching policy $\pi$ to a stationary caching policy $\pi^*$ equipped with the hindsight knowledge (\emph{i.e.,} $\pi^*$ knows the entire file-request sequence $\{\bm{x}_t\}_{1}^{T}$ in advance, \emph{viz.,} Eqns.\ \eqref{regret_seq}- \eqref{regret_def1}). Let $\bm{y}^j_*$ be the optimal stationary cache configuration vector at the server $j \in \mathcal{J}$ set by the policy $\pi^*$. Then the reward accrued by the fixed caching policy $\pi^*$ is given by: 
 \[ G_T^{\pi^{*}} = \sum_{t=1}^{T} \sum_{i \in \mathcal{I}} \bm{x}^i_t \cdot \sum_{j\in \partial^+(i)}\bm{y}_*^j.\]
%The regret $R_T$ is defined as follows:
%\[R_T = \sup_{\{\bm{x}_t^i\}}\sup_{\{\bm{y}_*^j\}} \bigg(\sum_{t=1}^{T} \sum_{i \in \mathcal{I}} \bm{x}^i_t \cdot \sum_{j\in \delta^+(i)}\bm{y}_*^j- \sum_{t=1}^{T} \sum_{i \in \mathcal{I}} \bm{x}^i_t \cdot \sum_{j\in \delta^+(i)}\bm{y}_t^j\bigg). \]
%Our objective in this section is to prove a lower bound for $R_T$. \\
Rearranging the terms, we have
%The optimal stationary cache configuration is easy to find. Rewrite 
\begin{eqnarray} \label{elastic_lb0}
 G_T^{\pi^*} = \sum_{j \in \mathcal{J}} \bm{y}_*^j\cdot \big( \sum_{i \in \partial^-(j)}\sum_{t=1}^{T} \bm{x}_t^i\big).
 \end{eqnarray}
Since the $j$\textsuperscript{th} cache has a total capacity of $C$, from the above equation, it is clear that the optimal stationary configuration $\bm{y}^j_*$ corresponds to caching the most frequent $C$ files requested by all of $j$'s in-neighbours taken together. 
%\textcolor{red}{See Figure []}.\\
%\paragraph{Regret lower bound:}
Following the probabilistic method described earlier for the proof of the single server regret bound (Theorem \ref{reg_lb_gnl}), we construct a randomized file-request sequence from the $i$\textsuperscript{th} user as follows: \[\bm{X}_t^{i} = \sum_{k=1}^{r} \bm{E}_{tk}^i, ~~i \in \mathcal{I},\] where the random variable $\bm{E}_{tk}^i$ is an $N$-dimensional unit vector, which is sampled independently and uniformly at random from the set of first $2C$ unit vectors $\{\bm{e}_i \in \mathbb{R}^N, 1\leq i \leq 2C\}$. Recall that, the unit vector $\bm{e}_i$ has one at its $i$\textsuperscript{th} coordinate and zeros everywhere else.
With this set up, the expected reward accrued by the policy $\pi$ (\emph{i.e.,} the second term in Eqn.\ \eqref{regret_seq}) may be computed as: 
\begin{eqnarray} \label{elastic_lb1}
&&\mathbb{E}\bigg( \sum_{t=1}^{T} \sum_{i \in \mathcal{I}} \bm{X}^i_t \cdot \sum_{j\in \partial^+(i)}\bm{Y}_t^j\bigg)\nonumber  \\
&=& \sum_{t=1}^{T} \sum_{i \in \mathcal{I}} \sum_{j \in \partial^+(i)} \sum_{f=1}^{N} \mathbb{E}(X^i_{tf})Y^j_{tf} \nonumber\\
&\stackrel{(a)}{=}& \frac{r}{2C} 	\sum_{t=1}^{T} \sum_{i \in \mathcal{I}} \sum_{j \in \partial^+(i)} \sum_{f=1}^{2C} Y^j_{tf} \nonumber \\
&\stackrel{(b)}{\leq} & \frac{r}{2C} \sum_{t=1}^{T} \sum_{i \in \mathcal{I}} \sum_{j \in \partial^+(i)} C 
\stackrel{(c)}{=}\frac{rT}{2}\sum_j d_j ,
\end{eqnarray}
where the Equation (a) follows from the fact that the random variables $\bm{X}_t$ and $\bm{Y}_t$ are independent and $\mathbb{E}(X^i_{tf})=\frac{r}{2C}, \forall i,t,f$. The inequality (b) follows from the cache-capacity constraints and finally, the equality (c) follows by changing the order of the summations. \\
%The quantity $d_j$ denotes the in-degree of the cache $j$ in the cache-network. \\
%Finally, we compute the expectation of the first term $G^{\pi^*}_T$. We have 
Finally, from Eqn.\ \eqref{elastic_lb0}, we compute the expected total reward $G^{\pi^*}_T$ accrued by the optimal stationary policy $\pi^*$: 
\begin{eqnarray*}
\mathbb{E}(G^{\pi^*}_T) = \sum_{j \in \mathcal{J}}  \mathbb{E}(M^j_C),
\end{eqnarray*}
where $M^j_C$ denotes the summation of $C$ highest coordinates of the $N$-dimensional random vector $\sum_{t=1}^{T} \sum_{i \in \delta^-(j)} \bm{X}_t^i$. Given the setup, the random variable $M_C$ is statistically identical to the total number of balls in the most occupied $C$ bins while $d_j rT$ balls are thrown independently and uniformly at random into $2C$ bins. Thus, using Lemma \ref{max_load}, we have 
\begin{eqnarray} \label{elastic_lb2}
\mathbb{E}(M^j_C) \geq \frac{rT}{2}d_j + \sqrt{\frac{d_jrCT}{2\pi}} - \Theta(\frac{1}{\sqrt{T}}). 	
\end{eqnarray}
Finally, combining Eqns.\ \eqref{elastic_lb1} and \eqref{elastic_lb2}, we have the following regret lower bound 
\begin{eqnarray*}
R^\pi_T \geq \sqrt{\frac{rCT}{2\pi}}\bigg(\sum_{j \in \mathcal{J}} \sqrt{d_j}\bigg) - \Theta(\frac{1}{\sqrt{T}}).	
\end{eqnarray*}
\end{proof}
\subsection{Proof of Theorem \ref{inelastic_th}} \label{reg_bd_inelastic}
\begin{proof}
We begin our analysis with the following two observations:
\begin{enumerate}
\item  From the definition of the reward functions \eqref{elastic_content} and \eqref{inelastic_content}, we have, in general, \[ q_{\textsf{inelastic}}(\bm{x}, \bm{y}) \leq q_{\textsf{elastic}}(\bm{x}, \bm{y}), ~~\forall \bm{x}, \bm{y}. \]
\item In the special case, when different servers $j \in \mathcal{J}$ cache \emph{different} items, \emph{i.e.,} $\bm{y}^i \cdot \bm{y}^j=0, \forall i\neq j$, we have 
\begin{eqnarray} \label{obs_2}
 q_{\textsf{inelastic}}(\bm{x}, \bm{y}) = q_{\textsf{elastic}}(\bm{x}, \bm{y}), ~~\forall \bm{x}, \bm{y}. 
 \end{eqnarray}
This follows from the fact that in the expression $ \bm{x}_t^i \cdot \big(\sum_{j \in \partial^+(i)} \bm{y}_t^j\big)= \sum_{j \in \partial^+(i)}\bm{x}_t^i \cdot \bm{y}_t^j$, only one of the dot-product terms could be strictly positive, since different servers caches different contents and $\bm{x}_t$ has only one positive component. Moreover, the value of each dot product is at most one, as each server stores at most one copy of each file.  
\end{enumerate}
With these two observations in mind, we now suitably modify the proof of the regret lower bound for elastic contents (Section \ref{reg_bd_elastic}) to obtain the corresponding regret lower bound for inelastic contents. As before, we construct a randomized file-request sequence $\{\bm{X}_t^i, i \in \mathcal{I}\}_{t\geq 1}$, where each of the random variable $\bm{X}_t^i$ is sampled independently and uniformly at random from the set of \emph{first} $2C|\mathcal{J}|$ unit vectors $\{\bm{e}_i \in \mathbb{R}^N, 1 \leq i \leq 2C|\mathcal{J}|\}$ (recall that, we assumed $r=1$ in this case).  Hence, using observation (1) and working similarly as in Eqn.\ \eqref{elastic_lb1}, the expected total reward $G_T^\pi$ accrued by any online caching policy may be upper bounded as 
\begin{eqnarray}\label{inelastic_lb1}
	G_T^\pi &\leq&\mathbb{E}\bigg( \sum_{t=1}^{T} \sum_{i \in \mathcal{I}} \bm{X}^i_t \cdot \sum_{j\in \partial^+(i)}\bm{Y}_t^j\bigg)\nonumber\\
	&\leq & \frac{T}{2|\mathcal{J}|}\sum_{j \in \mathcal{J}} d_j 	= \frac{Td}{2}.
\end{eqnarray}
For obtaining a lower bound to the total expected reward accrued by the optimal stationary policy $\pi^*$, in the following, we construct an $N|\mathcal{J}|$ dimensional stationary cache-configuration vector $\bm{Y}_*$ (obtained by stacking the $N$-dimensional cache-configuration vectors $\bm{Y}_*^j$ together $\forall j \in \mathcal{J}$) with the property that 
\begin{eqnarray}\label{zero_dot_product}
 \bm{Y}_*^i \cdot \bm{Y}_*^j =0, ~~ \forall i \neq j, ~~i, j \in \mathcal{J}. 
 \end{eqnarray}
\paragraph{Construction of the stationary cache configuration $\bm{Y}_\perp$:} The vectors $\{\bm{Y}_\perp^j, j \in \mathcal{J}\}$ are constructed sequentially, while always adhering to the property \eqref{zero_dot_product}. 
\begin{itemize}
\item The first vector $\bm{Y}_\perp^1$ is obtained by setting the coordinates corresponding to the top $C$ coordinates of the vector $\big( \sum_{i \in \partial^-(1)}\sum_{t=1}^{T} \bm{X}_t^i\big)$ to one and the rest to zero.  
\item Upon constructing the first $n-1$ vectors, the $n$\textsuperscript{th} stationary cache-configuration vector $\bm{Y}_\perp^n$ is constructed by setting the top $C$ coordinates of the random vector $\big( \sum_{i \in \partial^-(n)}\sum_{t=1}^{T} \bm{X}_t^i\big)$ to one which have not been set to one in any one of the previously constructed vectors $\{\bm{Y}_\perp^k, 1\leq k \leq n-1\}$, and the rest to zero.  
\end{itemize}
Clearly, the above construction ensures property \eqref{zero_dot_product}. 
For any vector $\bm{v}$, let the operator $S_v(m,n)$ denote the summation of coordinates running from $m$ to $n$ of the vector $\bm{v}$, sorted in non-increasing order. 
Define the random vector \[\bm{v}_j \equiv \sum_{i \in \partial^-(j)}\sum_{t=1}^{T} \bm{X}_t^i.\] A little thought reveals that, with the above construction, we have almost surely:
\begin{eqnarray} \label{inelastic_pf1}
 && \bm{Y}_\perp^j\cdot \bigg( \sum_{i \in \partial^-(j)}\sum_{t=1}^{T} \bm{X}_t^i\bigg) \nonumber \\
 &\geq& S_{\bm v_j}\bigg((j-1)C+1, jC \bigg),  ~~\forall j\in \mathcal{J}. 
 \end{eqnarray}  
Since the bipartite graph is assumed to be $d$-regular, and the random variables $\bm{X}_t^i$ are identically distributed, it is clear that the random vectors $\{\bm{v}_j, j \in \mathcal{J}\}$ are \emph{identically distributed} (note that, they are \emph{not} independent, in general).  
Finally, the reward accrued by the optimal stationary policy $\pi^*$ may be lower-bounded as:
\begin{eqnarray} \label{inelastic_star}
 G_T^{\pi^*} &\stackrel{(a)}{\geq}& \mathbb{E}\bigg( \sum_{j \in \mathcal{J}} \bm{Y}_\perp^j\cdot \big( \sum_{i \in \partial^-(j)}\sum_{t=1}^{T} \bm{X}_t^i\big) \bigg) \nonumber \\
 &\stackrel{(b)}{=}& \sum_{j \in \mathcal{J}} \mathbb{E}\bigg(\bm{Y}_\perp^j\cdot \big( \sum_{i \in \partial^-(j)}\sum_{t=1}^{T} \bm{X}_t^i\big) \bigg) 	\nonumber \\
 &\stackrel{(c)}{\geq}& \sum_{j \in \mathcal{J}} \mathbb{E}\bigg(S_{\bm v_j}\big( (j-1)C+1, jC\big) \bigg) \nonumber\\
 &\stackrel{(d)}{=}& \sum_{j \in \mathcal{J}} \mathbb{E}\bigg(S_{\bm v_1}\big( (j-1)C+1, jC\big) \bigg) \nonumber \\
  &=& \mathbb{E}\bigg(\sum_{j \in \mathcal{J}} S_{\bm v_1}\big( (j-1)C+1, jC\big) \bigg)\nonumber\\
  &=& \mathbb{E}\big(S_{\bm{v}_1}(1, |\mathcal{J}|C)\big) \nonumber\\
  &\stackrel{(e)}{\geq} & \frac{Td}{2} + \sqrt{\frac{d|\mathcal{J}|CT}{2\pi}} - \Theta(\frac{1}{\sqrt{T}}),
\end{eqnarray}
where the inequality (a) follows from Eqn.\ \eqref{obs_2} of observation 2, the equality (b) follows from the linearity of expectation, the inequality (c) follows from Eqn.\ \eqref{inelastic_pf1}, and the equation (d) follows from the fact that the r.v.s $\{\bm v_j, j \in \mathcal{J}\}$ are identically distributed. Finally, realize that the random variable $S_{\bm{v}_1}(1, |\mathcal{J}|C)$ is distributed as the total load of the most loaded $|\mathcal{J}|C$ bins when a total of $Td$ balls are thrown uniformly at random to $2 |\mathcal{J}|C$ bins. Hence, the inequality (e) follows from an application of Lemma \ref{max_load}. Finally, combining Eqns.\ \eqref{inelastic_lb1} and \eqref{inelastic_star}, we have 
\begin{eqnarray*}
R^\pi_T \geq G^{\pi^*}_T - G^{\pi}_T 
\geq \sqrt{\frac{d|\mathcal{J}|CT}{2\pi}} - \Theta(\frac{1}{\sqrt{T}}),	
\end{eqnarray*}
which concludes the proof. 
\end{proof}
